# Supplementary material for: 360DVD: Controllable Panorama Video Generation with 360-Degree Video Diffusion Model
Source: arXiv:2401.06578 source file (2024-05-10)
Supplement: Supplementary file 1 [file X_suppl.tex]

\clearpage
\setcounter{page}{1}
\maketitlesupplementary

\section{Additional Experimental Results}
\subsection{Continuity between Two Ends}
ERPs can be considered as the unfolding of a spherical surface along a meridian, thus, their left and right sides are meant to be continuous. We showcase the continuity at both ends of videos generated by our 360DVD and other compared approaches, as illustrated in Fig.~\ref{fig:continuity}. For ease of observation, we duplicated each video by concatenating it side by side twice. The portion highlighted with a red border in the middle represents the left-right connections. It can be observed that simply enabling the 360 Enhancement Techniques (360ET) during the inference phase significantly improves the continuity between the left and right ends of videos. When we further train on panorama video data and randomly rotate the training videos, we can achieve even more stable results, maintaining good left-right continuity in most scenes.

\begin{figure*}[b!]
    \centering
    \includegraphics[width=0.8\linewidth]{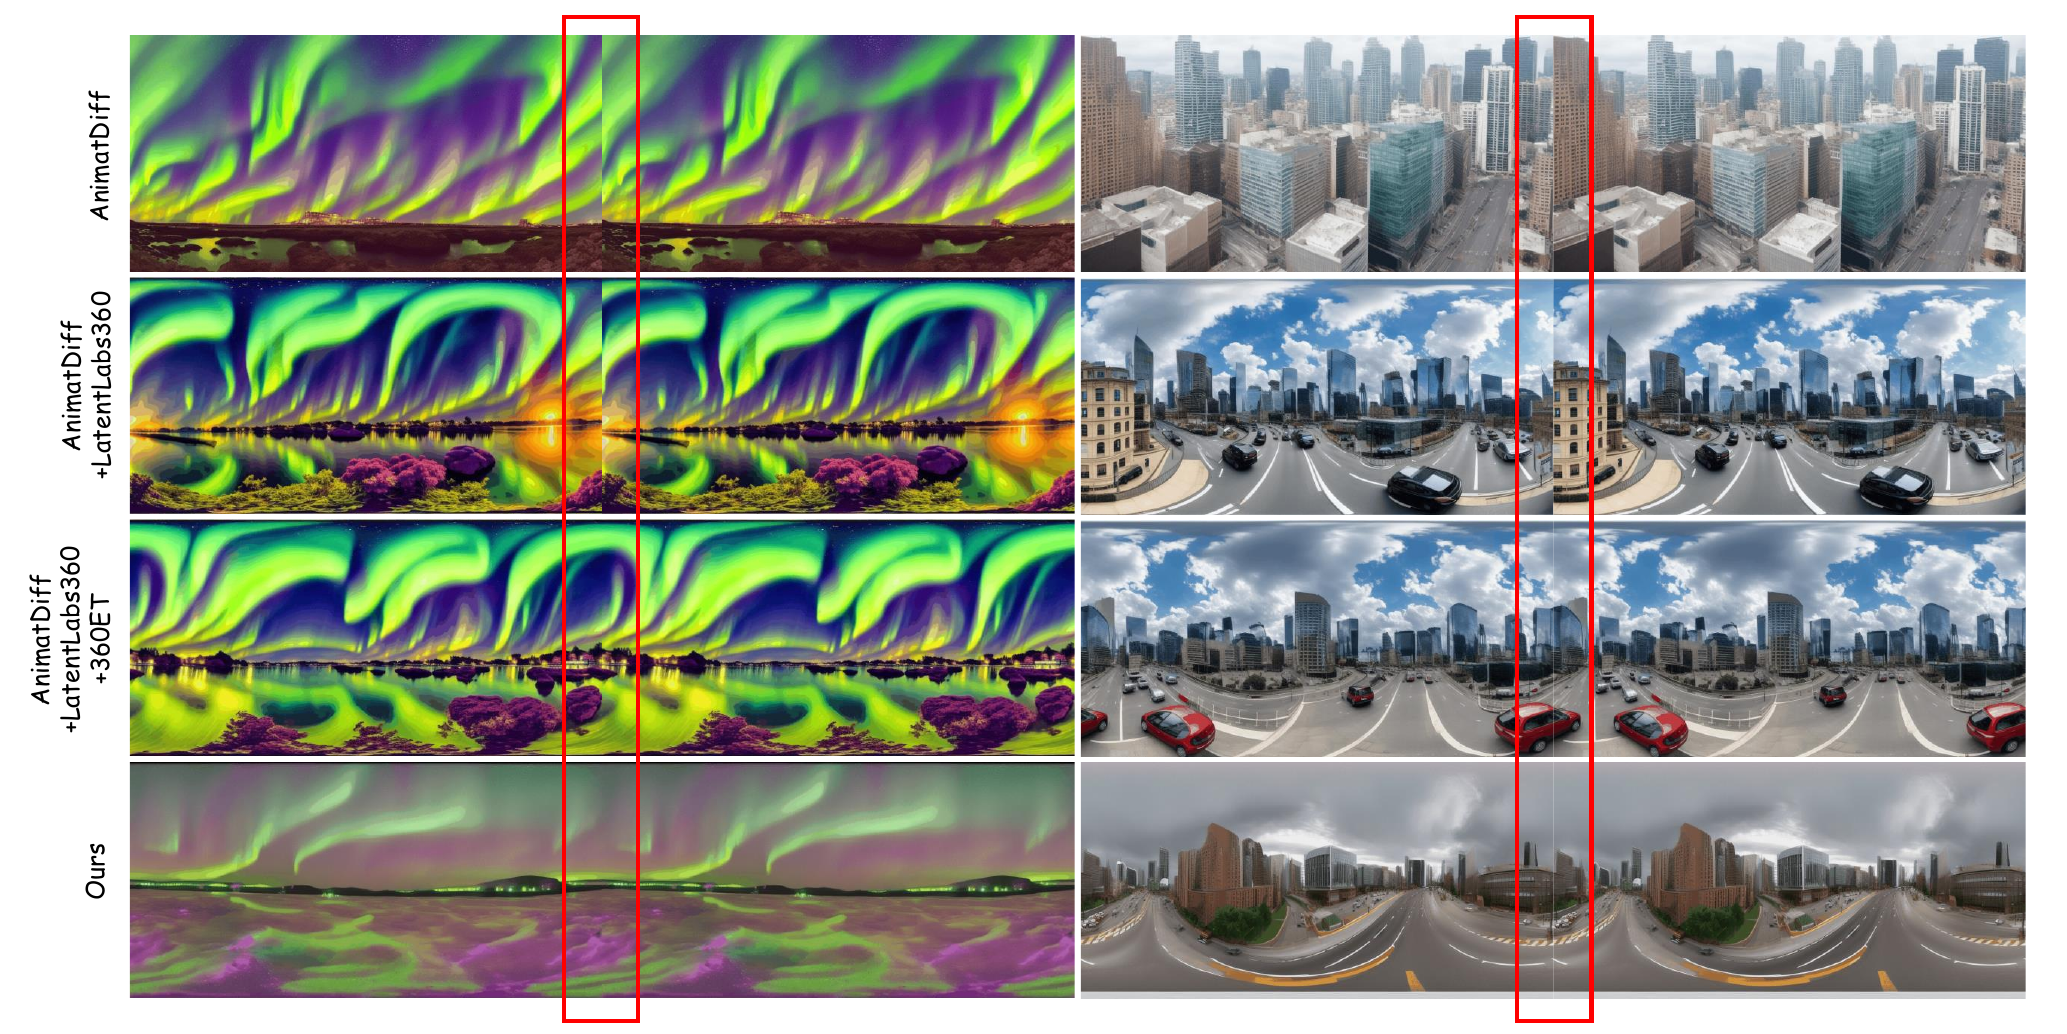}
    \caption{\textbf{Continuity between two ends} on videos generated by AnimateDiff, AnimateDiff with LatentLabs360, AnimateDiff with LatentLabs360 and 360 Enhancement Techniques (360ET), and ours 360DVD. The red box highlights the connection area.}
    \label{fig:continuity}
\end{figure*}

\begin{figure*}[htbp]
    \centering
    \includegraphics[width=0.9\linewidth]{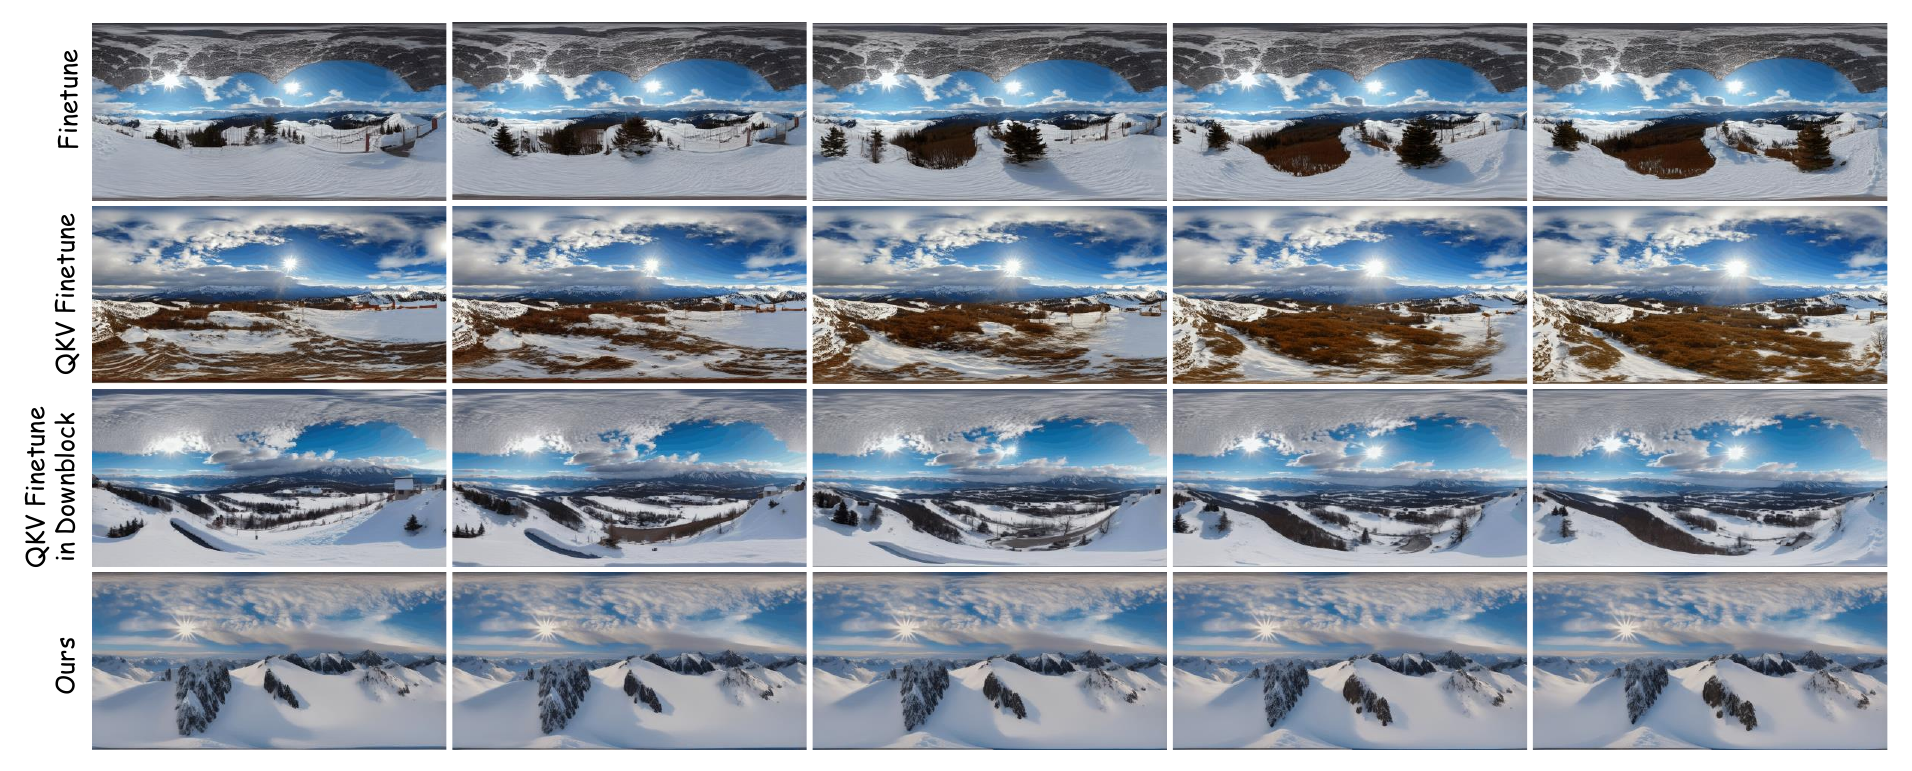}
    \caption{\textbf{Training Strategy.} Compared to fine-tuning the Motion Module, 360DVD achieves better video quality and more stable motion.}
    \label{fig:finetune}
\end{figure*}

\begin{figure*}[htbp]
    \centering
    \includegraphics[width=0.8\linewidth]{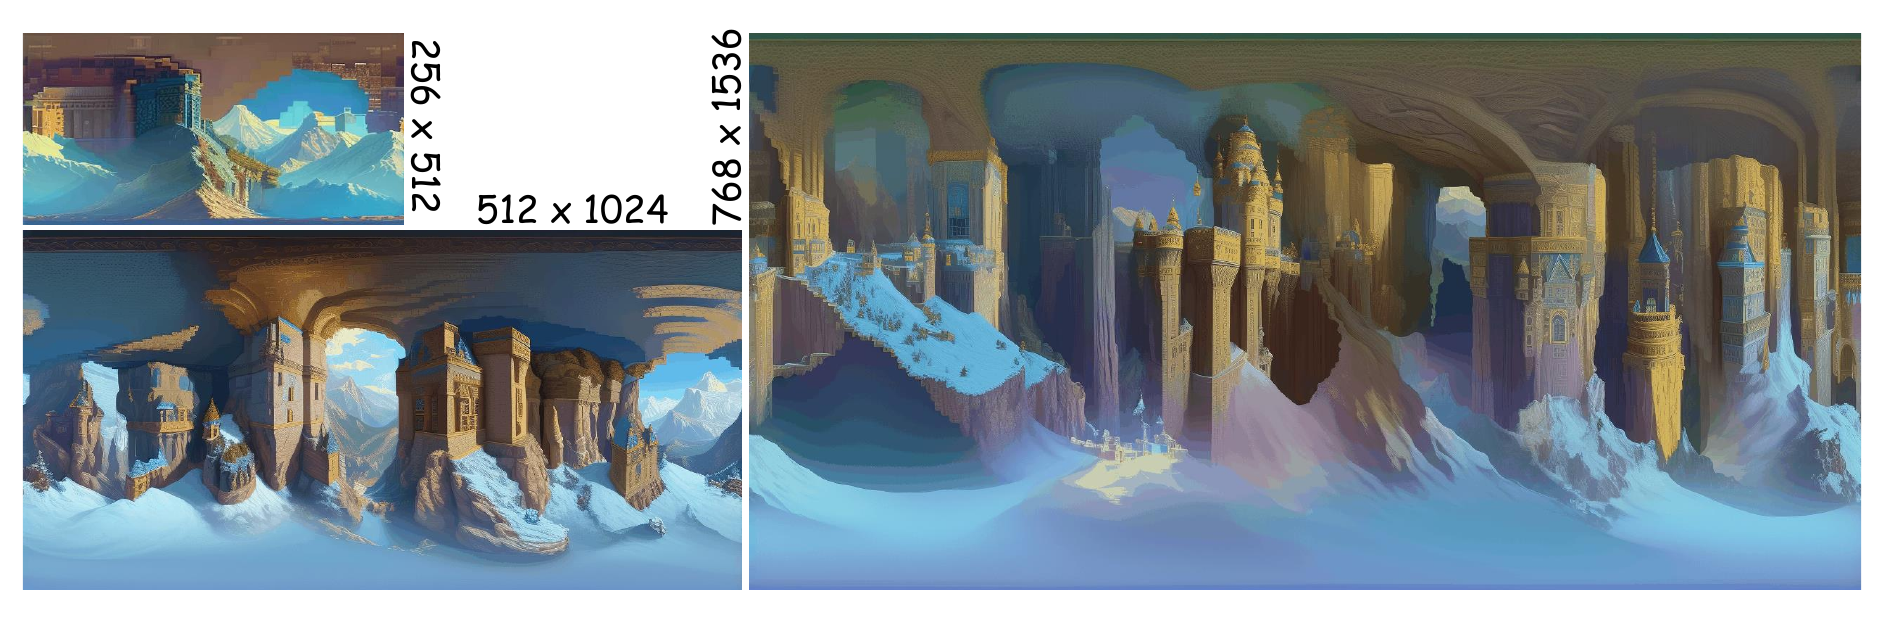}
    \caption{\textbf{Scalability.} Results at different resolutions demonstrate the generalization of our method.}
    \label{fig:scalab}
\end{figure*}

\subsection{Adapter vs. Finetune}
While fine-tuning AnimateDiff may seem like a simpler and more intuitive approach, in practice, we found that the results generated by the fine-tuned model were not satisfactory as shown in Fig.~\ref{fig:finetune}. We attempted three fine-tuning methods: fine-tuning all the Motion Module parameters, fine-tuning only the QKV parameters in the Motion Module, and fine-tuning the Motion Module parameters in the downblock of the Motion Module. Although they managed to learn some aspects of the content distribution and motion patterns in panorama videos, they exhibited noticeable issues such as occasional artifacts in the sky and significant flickering due to large motion amplitudes. More importantly, these methods cannot accept motion control as the condition. On the contrary, training an additional Adapter provides more flexibility to adjust the model's structure and parameters, better adapting it to the requirements of panoramic video generation. 

\subsection{Scalability}
Although our method is trained at a resolution of $512 \times 1024$, it also generalizes well at other resolutions as presented in Fig.~\ref{fig:scalab}.

\subsection{Influence of 360 Adapter}
The condition feature extraction and conditioning operation of the 360-Adapter is defined as:
\begin{equation}
    F_c = \mathcal{F}_{360}(C),
\end{equation}
\begin{equation}
    \hat{F}^i_{enc} = F^i_{enc} + F^i_c, i \in \{1, 2, 3, 4\},
    \label{eq:adapter}
\end{equation}
where $C$ is motion conditions, $\mathcal{F}_{360}(\cdot)$ is 360-Adapter, and $F_c$ are the feature maps  generated by 360-Adapter.

We can adjust the influence of the 360 Adapter on the video generation process by introducing an additional hyper-parameter weight $w$. Then, the conditioning operation can be re-written into: 
\begin{equation}
    \hat{F}^i_{enc} = F^i_{enc} + w F^i_c, i \in \{1, 2, 3, 4\}.
    \label{eq:adapter}
\end{equation}

As illustrated in Fig.~\ref{fig:weight}, when $w$ is set to 0, the video generation pipeline is not modulated, only the AnimateDiff works. As the weight increases, the content distribution of the generated videos more closely aligns with panoramic characteristics, and the control ability of the input motion condition on video motion becomes stronger.

\subsection{Results on Sphere Surface}
In Fig.~\ref{fig:sphere}, we present the results of projecting the generated videos in ERP format back onto the sphere surface. Our approach can produce high-quality results from various perspectives. Compared to generating individual perspectives and then merging them into a panorama, directly generating panorama videos achieves more consistent content and style. We recommend seeing the videos on the webpage we provided in supplementary material.

\section{Limitations}
In this paper, we have proposed a simple yet effective baseline named 360DVD for $360^{\circ}$ panorama video generation. However, there are still some limitations. Firstly, its performance depends on the underlying method for regular video generation, as these parameters are frozen during training. While this ensures that their generation capability is preserved, it also limits the capabilities of our method. Secondly, the motion conditions of the training data are predicted using a panoramic optical flow estimator, and the performance of existing panoramic optical flow estimators is limited, resulting in suboptimal flow pairs that, to some extent, affect our performance. Thirdly, we have only attempted control effects using optical flow and have not tested it on other motion conditions such as depth maps. We leave this as future work.

\begin{figure*}[htbp]
    \centering
    \includegraphics[width=1.0\linewidth]{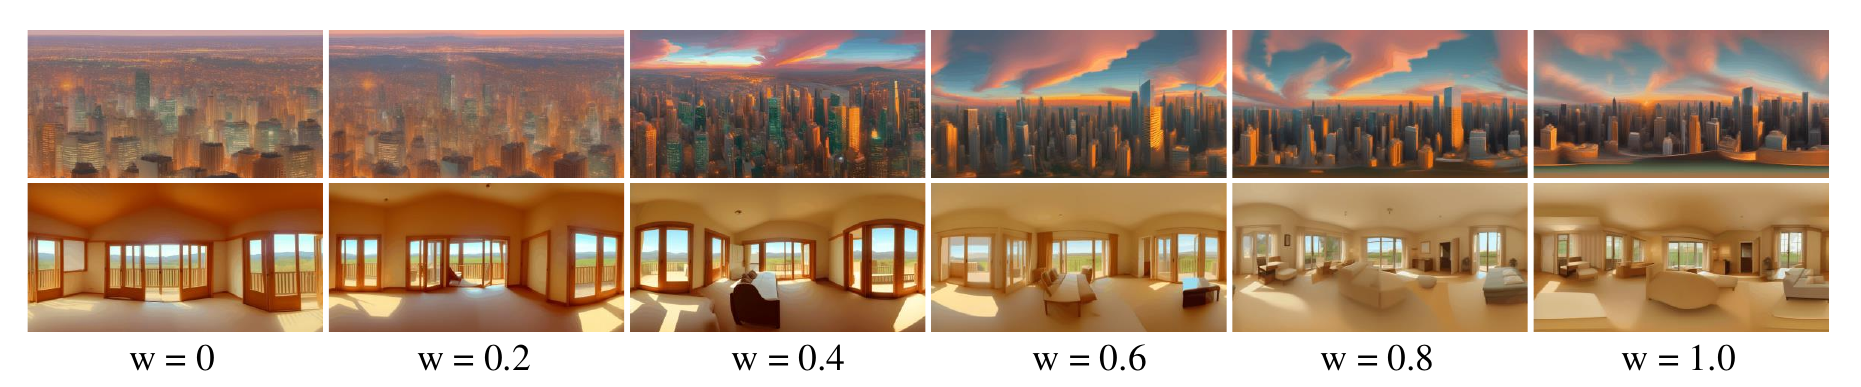}
    \caption{\textbf{Influence of 360 Adapter.} A larger weight $w$ of 360 Adapter leads to a more pronounced panoramic effect, enhancing the control of motion conditions.}
    \label{fig:weight}
\end{figure*}

\begin{figure*}[htbp]
    \centering
    \includegraphics[width=0.9\linewidth]{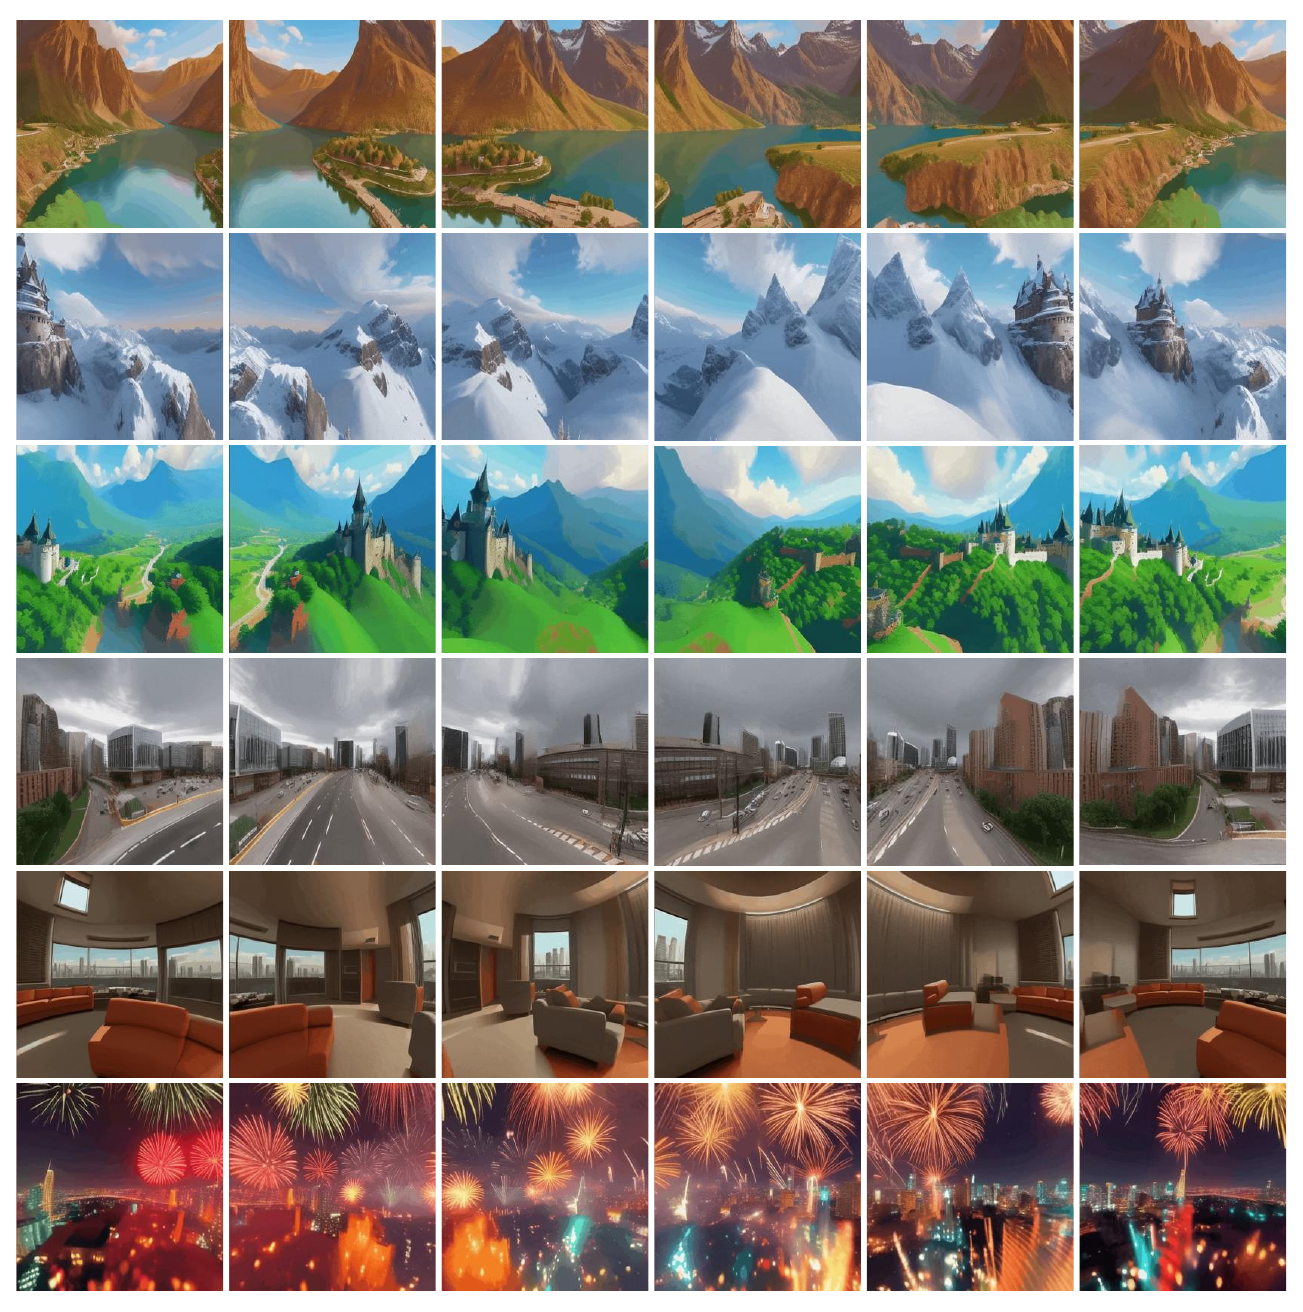}
    \caption{\textbf{Results on Sphere Surface.} The generated ERPs are projected back onto the sphere surface and captured from a partial angle.}
    \label{fig:sphere}
\end{figure*}

% \section{Rationale}
% \label{sec:rationale}
% % 
% Having the supplementary compiled together with the main paper means that:
% % 
% \begin{itemize}
% \item The supplementary can back-reference sections of the main paper, for example, we can refer to \cref{sec:intro};
% \item The main paper can forward reference sub-sections within the supplementary explicitly (e.g. referring to a particular experiment); 
% \item When submitted to arXiv, the supplementary will already included at the end of the paper.
% \end{itemize}
% % 
% To split the supplementary pages from the main paper, you can use \href{https://support.apple.com/en-ca/guide/preview/prvw11793/mac#:~:text=Delete%20a%20page%20from%20a,or%20choose%20Edit%20%3E%20Delete).}{Preview (on macOS)}, \href{https://www.adobe.com/acrobat/how-to/delete-pages-from-pdf.html#:~:text=Choose%20%E2%80%9CTools%E2%80%9D%20%3E%20%E2%80%9COrganize,or%20pages%20from%20the%20file.}{Adobe Acrobat} (on all OSs), as well as \href{https://superuser.com/questions/517986/is-it-possible-to-delete-some-pages-of-a-pdf-document}{command line tools}.
